# Supplementary material for: Magnetic field resilient superconducting coplanar waveguide resonators for hybrid cQED experiments
Source: arXiv:1809.03932 ancillary file (2018-09-11)
Supplement: Supplementary file 1 [file Supplementary.pdf]

# Supplementary Material:

## Magnetic field resilient superconducting coplanar waveguide resonators for hybrid cQED experiments

J. G. Kroll,<sup>1,2</sup> F. Borsoi,<sup>1,2</sup> K. L. van der Enden,<sup>1,2</sup> W. Uilhoorn,<sup>1,2</sup> D. de Jong,<sup>1,2</sup>  
M. Quintero-Pérez,<sup>1,3</sup> D. J. van Woerkom,<sup>1,2</sup> A. Bruno,<sup>1,2</sup> S. R. Plissard,<sup>4,\*</sup> D.  
Car,<sup>4</sup> E. P. A. M. Bakkers,<sup>4</sup> M. C. Cassidy,<sup>1,2,†</sup> and L. P. Kouwenhoven<sup>1,2,5,‡</sup>

<sup>1</sup>*QuTech, Delft University of Technology, Delft, 2600 GA, The Netherlands*

<sup>2</sup>*Kavli Institute for Nanoscience, Delft University of Technology, Delft, 2600 GA, The Netherlands*

<sup>3</sup>*Netherlands Organisation for Applied Scientific Research (TNO), Delft, 2600 AD, The Netherlands*

<sup>4</sup>*Department of Applied Physics, Eindhoven University of Technology, Eindhoven, 5600 MB, The Netherlands*

<sup>5</sup>*Microsoft Station Q Delft, Delft, 2600 GA, The Netherlands*

(Dated: September 11, 2018)

### I. DEVICE PARAMETERS

A large number of devices were fabricated and measured in the creation of this manuscript. Table S1 contains the important physical parameters for all resonators used in this paper.

| Film | $t$ (nm) | Device | Resonator | Type        | $S$ ( $\mu\text{m}$ ) | $W$ ( $\mu\text{m}$ ) | $L$ ( $\mu\text{m}$ ) | $f_r$ (GHz) | $\rho_h$ ( $\mu\text{m}^{-1}$ ) | $B_{\text{Th}}$ (mT) |
|------|----------|--------|-----------|-------------|-----------------------|-----------------------|-----------------------|-------------|---------------------------------|----------------------|
| 1    | 8        | 1      | 1         | $\lambda/4$ | 42                    | 0.4                   | 2124                  | 6.037       | 0                               | 0                    |
| 2    | 22       | 2      | 1         | $\lambda/4$ | 32                    | 2.5                   | 3780                  | 5.485       | 0                               | 0                    |
| 3    | 100      | 3      | 1         | $\lambda/4$ | 15                    | 4                     | 4443                  | 5.927       | 0                               | 0                    |
| 4    | 300      | 4      | 1         | $\lambda/4$ | 11.5                  | 4                     | 5935                  | 4.953       | 0                               | 0                    |
| 2    | 22       | 5      | 1         | $\lambda/4$ | 4                     | 10                    | 1969                  | 7.994       | 0                               | 0                    |
| 2    | 22       | 5      | 2         | $\lambda/4$ | 4                     | 10                    | 2652                  | 5.854       | 1.8                             | 3.7                  |
| 2    | 22       | 5      | 3         | $\lambda/4$ | 4                     | 10                    | 2542                  | 5.995       | 4.6                             | 9.6                  |
| 2    | 22       | 5      | 4         | $\lambda/4$ | 4                     | 10                    | 2441                  | 6.109       | 7.2                             | 14.9                 |
| 2    | 22       | 5      | 5         | $\lambda/4$ | 4                     | 10                    | 2104                  | 6.786       | 12.8                            | 26.5                 |
| 2    | 22       | 5      | 6         | $\lambda/4$ | 4                     | 10                    | 2034                  | 5.971       | 28.9                            | 59.7                 |
| 2    | 22       | 6      | 1         | $\lambda/4$ | 8                     | 1                     | 2760                  | 4.873       | 1.2                             | 2.5                  |
| 2    | 22       | 6      | 2         | $\lambda/4$ | 8                     | 5                     | 3180                  | 5.106       | 1.2                             | 2.5                  |
| 2    | 22       | 6      | 3         | $\lambda/4$ | 8                     | 10                    | 3277                  | 5.347       | 1.2                             | 2.5                  |
| 2    | 22       | 6      | 4         | $\lambda/4$ | 4                     | 1                     | 2038                  | 5.587       | 1.2                             | 2.5                  |
| 2    | 22       | 6      | 5         | $\lambda/4$ | 4                     | 5                     | 2411                  | 5.773       | 1.2                             | 2.5                  |
| 2    | 22       | 6      | 6         | $\lambda/4$ | 4                     | 10                    | 2503                  | 5.98        | 1.2                             | 2.5                  |
| 2    | 22       | 6      | 7         | $\lambda/4$ | 2                     | 10                    | 1832                  | 5.984       | 1.2                             | 2.5                  |
| 2    | 22       | 6      | 8         | $\lambda/4$ | 2                     | 1                     | 1904                  | 6.063       | 1.2                             | 2.5                  |
| 2    | 22       | 6      | 9         | $\lambda/4$ | 2                     | 5                     | 1534                  | 6.091       | 1.2                             | 2.5                  |
| 2    | 22       | 6      | 10        | $\lambda/4$ | 1                     | 1                     | 1172                  | 6.133       | 1.2                             | 2.5                  |
| 2    | 22       | 6      | 11        | $\lambda/4$ | 1                     | 5                     | 1391                  | 6.271       | 1.2                             | 2.5                  |
| 2    | 22       | 6      | 12        | $\lambda/4$ | 1                     | 10                    | 1443                  | 6.427       | 1.2                             | 2.5                  |
| 5    | 20       | 7      | 1         | $\lambda/2$ | 10                    | 1.5                   | 6650                  | 4.992       | 3.6                             | 6.6                  |
| 2    | 22       | 8      | 1         | $\lambda/4$ | 16                    | 0.4                   | 3335                  | 3.529       | 0                               | 0                    |
| 2    | 22       | 8      | 2         | $\lambda/4$ | 8                     | 0.4                   | 2914                  | 3.956       | 0                               | 0                    |
| 2    | 22       | 8      | 3         | $\lambda/4$ | 4                     | 0.4                   | 2685                  | 3.974       | 0                               | 0                    |
| 2    | 22       | 8      | 4         | $\lambda/4$ | 2                     | 0.4                   | 2453                  | 4.419       | 0                               | 0                    |
| 2    | 22       | 8      | 5         | $\lambda/4$ | 16                    | 0.4                   | 2732                  | 4.498       | 0                               | 0                    |
| 2    | 22       | 8      | 6         | $\lambda/4$ | 8                     | 0.4                   | 2553                  | 4.534       | 0                               | 0                    |
| 2    | 22       | 8      | 7         | $\lambda/4$ | 4                     | 0.4                   | 2373                  | 5.054       | 0                               | 0                    |
| 2    | 22       | 8      | 8         | $\lambda/4$ | 2                     | 0.4                   | 2188                  | 5.567       | 0                               | 0                    |

TABLE S1. Table of important physical parameters for all devices.

\* Current address: CNRS, LAAS-CNRS, Universit de Toulouse, 31400 Toulouse, France

† Current address: Microsoft Station Q Sydney, Sydney, NSW 2006, Australia

‡ Leo.Kouwenhoven@Microsoft.com

## II. FITTING PROCEDURE

To accurately extract the  $Q_i$  of our  $\lambda/4$  resonators at single photon levels we follow the fitting procedure detailed in [1, 2]. The complex transmission parameter  $S_{21}$  is fitted with the following formula:

$$S_{21} = A \left( 1 + \alpha \frac{f - f_r}{f_r} \right) \left( 1 - \frac{\frac{Q_l}{|Q_e|} e^{i\theta}}{1 + 2iQ_l \frac{f - f_r}{f_r}} \right) e^{i\theta_r f + \phi_0} \quad (1)$$

Where  $A$  is the amplitude of the bare feedline transmission in the absence of a resonance,  $\alpha$  is a background slope parameter to account for non-uniform background transmission,  $f$  is the probe frequency,  $f_r$  is the resonance frequency,  $Q_l$  is the loaded quality factor,  $Q_e$  is a complex-valued external quality factor related to  $Q_e$  via  $1/Q_e = \text{Re}(1/Q_e)$  and  $\phi_0$  and  $\phi_e$  compensate for signal propagation delays to and from the sample.

For the  $\lambda/2$  resonators without a calibration of the baseline transmission  $Q_i$  cannot be accurately extracted. In this case we extract only  $Q_l$  by fitting  $S_{21}$  using:

$$S_{21} = A \frac{\delta f}{(f - f_r)^2 + (\delta f^2/4)} \quad (2)$$

Where  $A$  is the amplitude of the Lorentzian,  $\delta f$  is the full width half maximum of the resonance,  $f$  is the probe frequency and  $f_r$  is the resonance frequency. The quality factor is defined to be  $Q_l = f_r/\delta f$ .

## III. CALCULATION OF KINETIC INDUCTANCE FRACTION $\alpha$

The kinetic inductance fraction  $\alpha$  is used to represent how strongly the kinetic inductance  $L_k$  contributes to the total waveguide inductance  $L_t$ , given by  $\alpha = L_k/L_t$ . To determine  $\alpha$  we first consider how the resonance frequency  $f_r$  is set in a distributed element LC resonator model:

$$f_r = \frac{1}{4l\sqrt{LC}} \quad (3)$$

Where  $f_r$  is the resonance frequency,  $l$  is the resonator length,  $C$  is the capacitance per unit length and  $L$  is the inductance per unit length of the resonator. The total inductance  $L_t$  consists of a contribution from the kinetic inductance  $L_k$  and a contribution from the geometry  $L_g$  summing to give  $L_t = L_k + L_g$ . We use geometric models to estimate  $C$  and  $L_g$  of the CPW resonator [3]:

$$L_g = \frac{\mu_0}{4} \frac{K(k')}{K(k)} l \quad (4)$$

$$C = 4\epsilon_0\epsilon_{\text{eff}} \frac{K(k)}{K(k')} l \quad (5)$$

Where  $\mu_0$  is the permeability of free space,  $\epsilon_0$  is the permittivity of free space,  $\epsilon_{\text{eff}}$  is the effective dielectric constant of the CPW,  $K$  is the complete elliptic integral of the first kind and  $k$  is the fraction of the central conductor to the total CPW width.  $k = S/(S + 2W)$  where  $S$  is the width of the central conductor and  $W$  is the width of the gap between the central conductor and the ground plane.

Rearranging to extract  $L_k$ :

$$L_k = \frac{1}{16f_r^2 l^2 C} - L_g \quad (6)$$

Allowing  $\alpha$  to be defined as:

$$\alpha = \frac{1 - 16f_r^2 l^2 C L_g}{1} \quad (7)$$

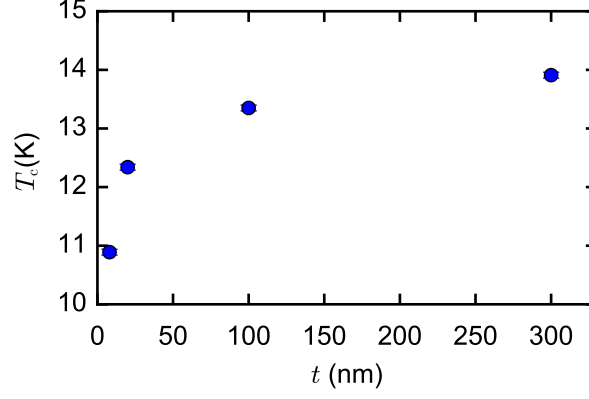

FIG. S1. Critical temperature  $T_c$  of NbTiN films as a function of  $t$ .

#### IV. SUPERCONDUCTING CRITICAL TEMPERATURE OF NBTIN FILMS

Prior to fabricating devices, the superconducting critical temperature ( $T_c$ ) of each film was measured. Thicknesses  $t$  ranged from 8 nm to 300 nm. We found  $T_c$  to monotonically increase as a function of the thickness reaching a maximum for  $t = 300$  nm (Fig. S1). As  $t$  approaches the superconducting coherence length  $\xi$  of the material,  $T_c$  is strongly reduced. From this we infer that the superconducting gap  $\Delta$  is also reduced.

#### V. HOLEY GROUND PLANE

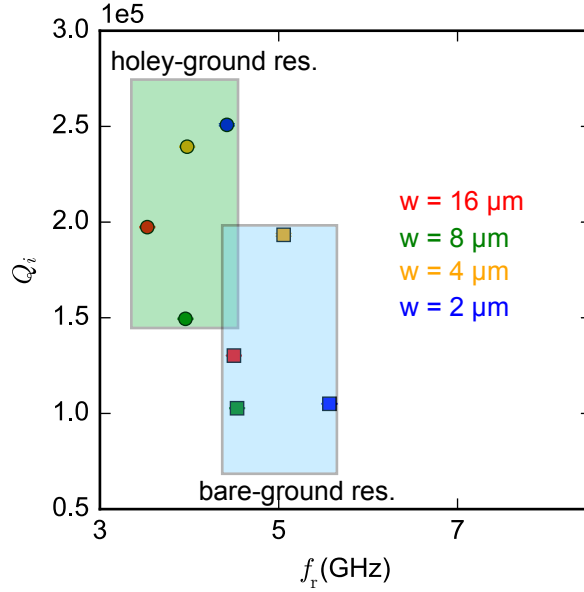

FIG. S2. Role of the holey ground at  $B = 0$  T:  $Q_i$  as a function of resonant frequency with different colors for varying central conductor widths ( $S$ ) in device 8. The gap ( $W$ ) of all resonators is  $0.4 \mu\text{m}$ . Scatter points in the transparent green (blue) box are for holey-ground (bare-ground) resonators.

In addition to an array of small holes that pin vortices around the CPW of resonators in devices 5, 6 and 7, the ground plane of these devices were also covered in large holes that were designed to trap residual magnetic fluxes that occur in the laboratory environment when (nominally) at  $B = 0$  T. To test what effect, if any, this had on the

$Q_i$  of resonators, we fabricated a device ( $t = 22$  nm) hosting 8 resonators multiplexed to a common feedline. Half of these resonators were patterned with a holey ground plane and half with a bare ground plane with no holes. In this device the holey ground consists of etched squares  $1\text{ }\mu\text{m} \times 1\text{ }\mu\text{m}$  separated by superconducting strips  $1\text{ }\mu\text{m}$  wide. The resonator geometries were varied by modifying the width of the central conductor (Table S1, device 8, resonators 1 to 8), and contained no holes around the CPW.

The device was cooled down to base temperature 3 times. Resonators on holey ground were stable, whereas those on bare ground exhibited small fluctuations in  $f_r$ , giving distorted line shapes. Upon application of a small parallel magnetic field  $B_{\parallel} \simeq 0.1$  mT all resonators were found to become unstable, demonstrating the importance of holes around the CPW for preserving the resonator's performance in parallel magnetic fields. The  $Q_i$ s of resonators with the same  $W$  at  $B = 0$  T are higher if they are surrounded by holey ground (see Fig. S2). To fully validate this observation a more detailed study is required. Additionally the  $f_r$  of each resonator without holey ground was found to vary significantly on each cool down, providing evidence that a small number of vortices were trapped around the CPW of each resonator.

## VI. FIELD ALIGNMENT PROCEDURE

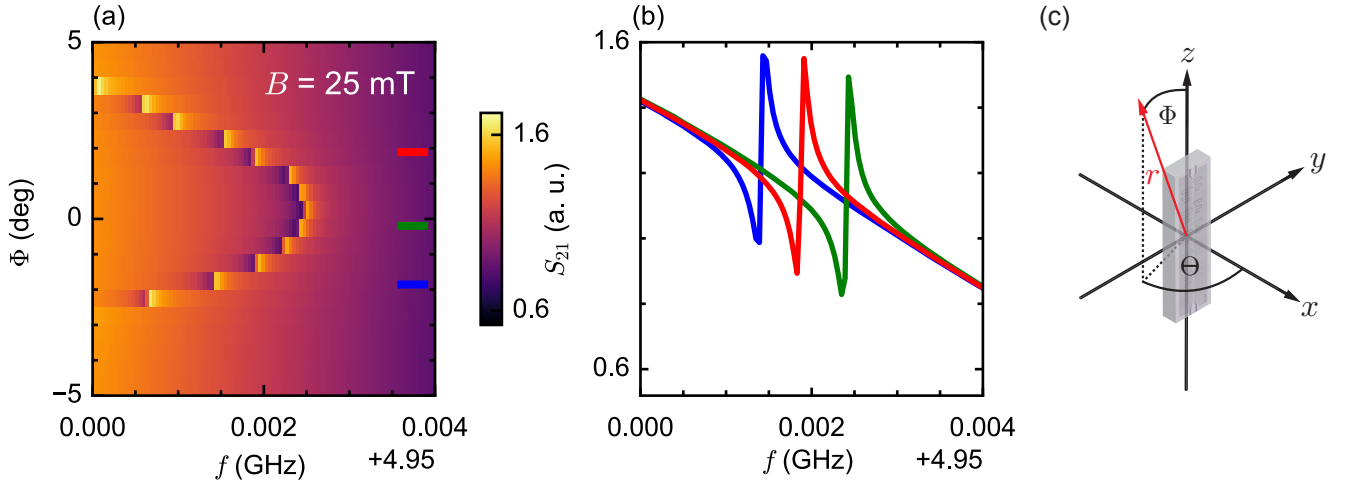

FIG. S3. Field alignment procedure at  $B = 25$  mT: (a) shift of the  $f_r$  as a function of  $\Phi$  for resonator 1 in device 4 ( $t = 300$  nm), where  $\Phi$  is the spherical angle with respect to the plane of the film. (b) Three representative linecuts. In this case, the optimal  $\Phi$  is  $-0.3$  deg. (c) Coordinate system used throughout the paper for each device. At  $\Theta = 0$  the angle  $\Phi$  is only relative to the plane of the film.

An accurate alignment of the magnetic field direction with respect to the plane of the film was required to minimise the nucleation of vortices in the superconductor. After setting the field magnitude to the required value, the spherical angle  $\phi$  was fine tuned and the response of the resonant frequency monitored. As the perpendicular component of the magnetic field causes the frequency to decrease faster than the parallel one, we optimised the angle for in-plane measurements to maximise the frequency and minimise the number of vortices present in the device (Fig. S3).

## VII. RESONATORS WITH HOLES IN PARALLEL MAGNETIC FIELD

Here we report the response of the 11 other resonators on device 6 (See Tab. S1) with holes studied in parallel magnetic field. These are patterned on a  $t = 22$  nm thick film with a hole density of  $\rho_h = 1.2\text{ }\mu\text{m}^{-2}$ . Each hole has a diameter of 300 nm. The 12 resonators were designed to have different geometries; in particular, we varied the width of the central conductor ( $S$ ) and the gap ( $W$ ) between the central conductor and the ground plane. In the main text

(see Fig. 4) we report the response of resonator 1. Our measurements did not indicate that the geometry plays an important role in protecting the resonators from nucleation of vortices. In fact we found that - with holes - both the frequency shift and the internal quality factor of all resonators have similar trend in parallel magnetic field (Fig. S4).

- 
- [1] M S Khalil, M. J.A. Stoutimore, F C Wellstood, and K D Osborn. An analysis method for asymmetric resonator transmission applied to superconducting devices. *Journal of Applied Physics*, 111(5), 2012.
  - [2] A. Bruno, G. De Lange, S. Asaad, K. L. Van Der Enden, N. K. Langford, and L. Dicarlo. Reducing intrinsic loss in superconducting resonators by surface treatment and deep etching of silicon substrates. *Applied Physics Letters*, 106(18):182601, may 2015.
  - [3] R. Barends. Photon-detecting superconducting resonators, 2009.

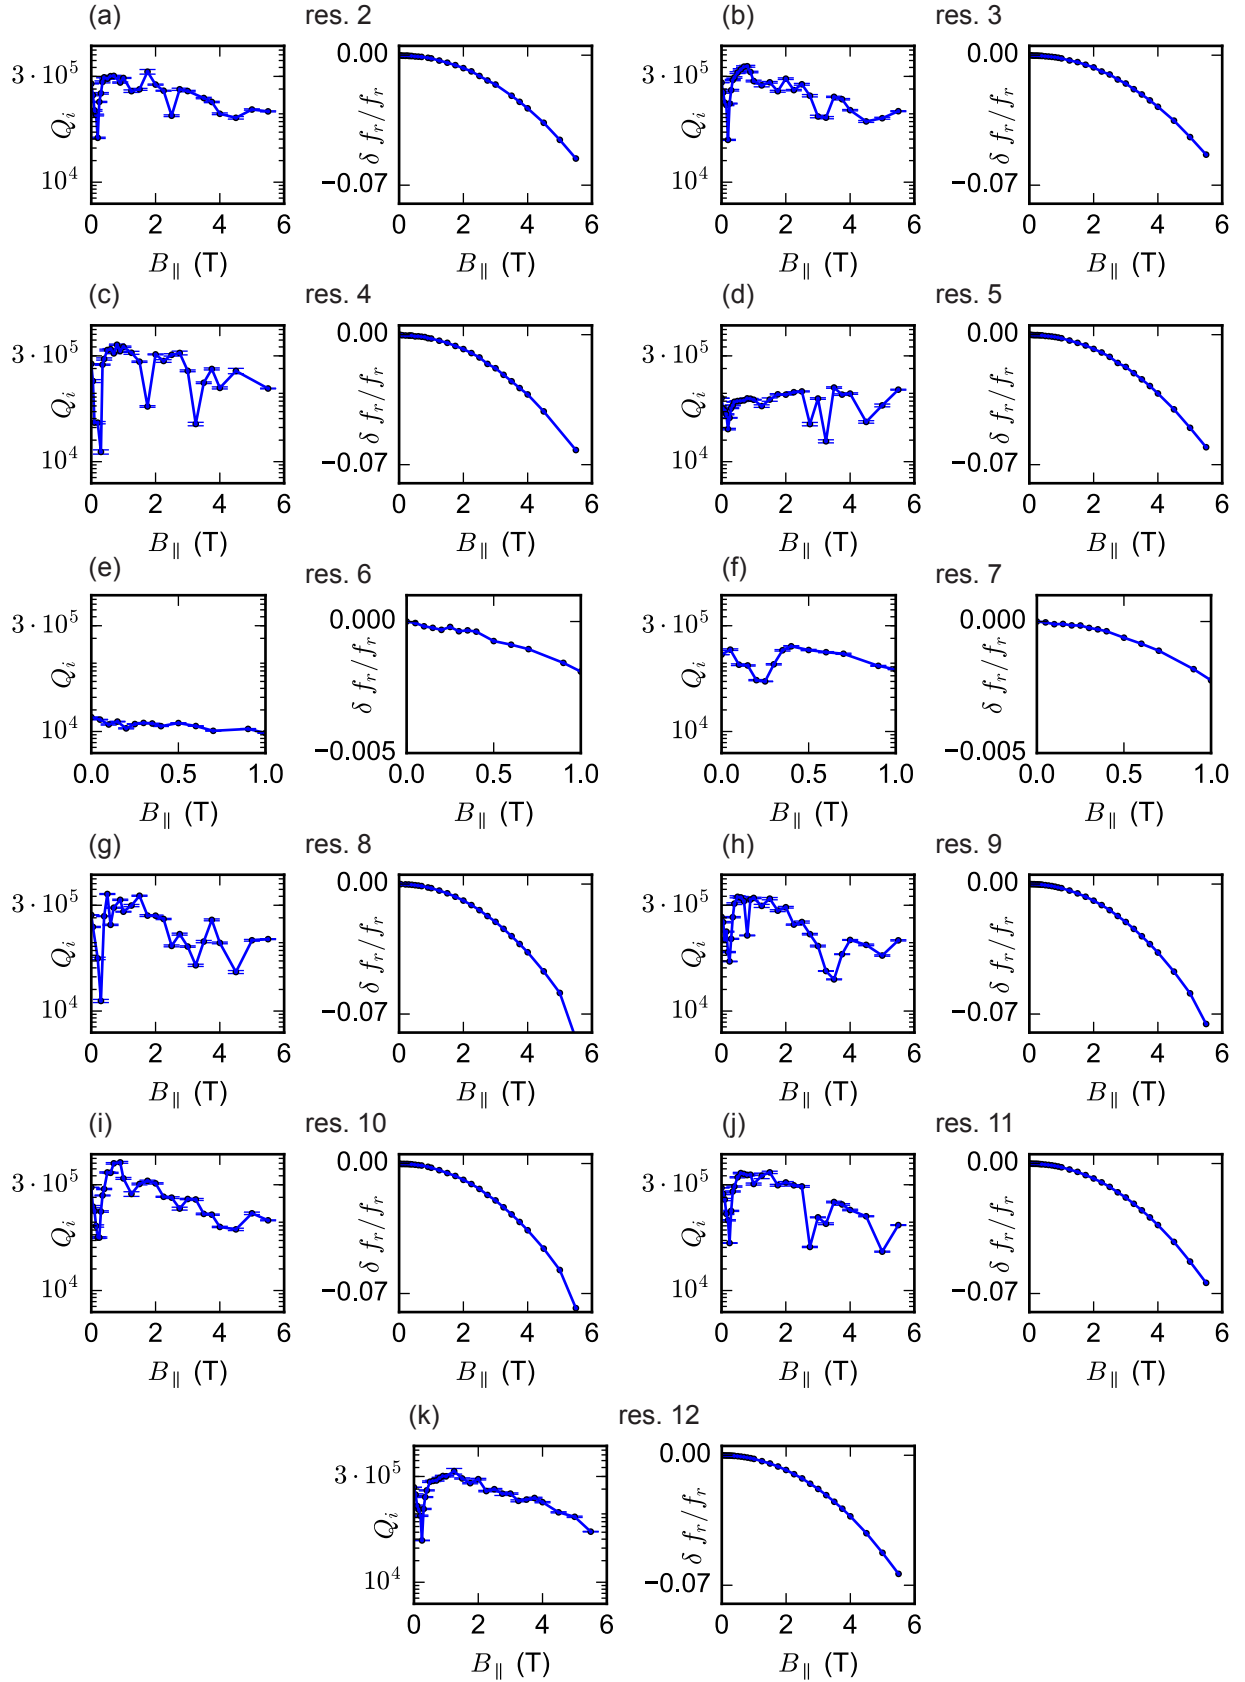

FIG. S4. Resonators with holes in parallel magnetic field: from (a) to (k) the relative frequency shift ( $\delta f_r / f_r(B)$ ) and  $Q_i(B)$  for resonators 2 to 12 in device 6. Resonators 6 and 7 could not be investigated above  $B = 1$  T as their  $f_r$  overlapped.
